# Supplementary material for: EditScout: Locating Forged Regions from Diffusion-based Edited Images with Multimodal LLM
Source: arXiv:2412.03809 source file (2024-12-05)
Supplement: Supplementary file 1 [file 6_supp.tex]

% \appendix

\section{Appendix / supplemental material}
\subsection{Datasets}

\subsection{Implementation details}

\subsection{Qualitative results}
